# Supplementary material for: Effective Rotation-invariant Point CNN with Spherical Harmonics kernels
Source: arXiv:1906.11555 source file (2019-09-10)
Supplement: Supplementary file 1 [file appendix.tex]

\begin{figure*}[h!]
    \centering
     \includegraphics[width=17cm]{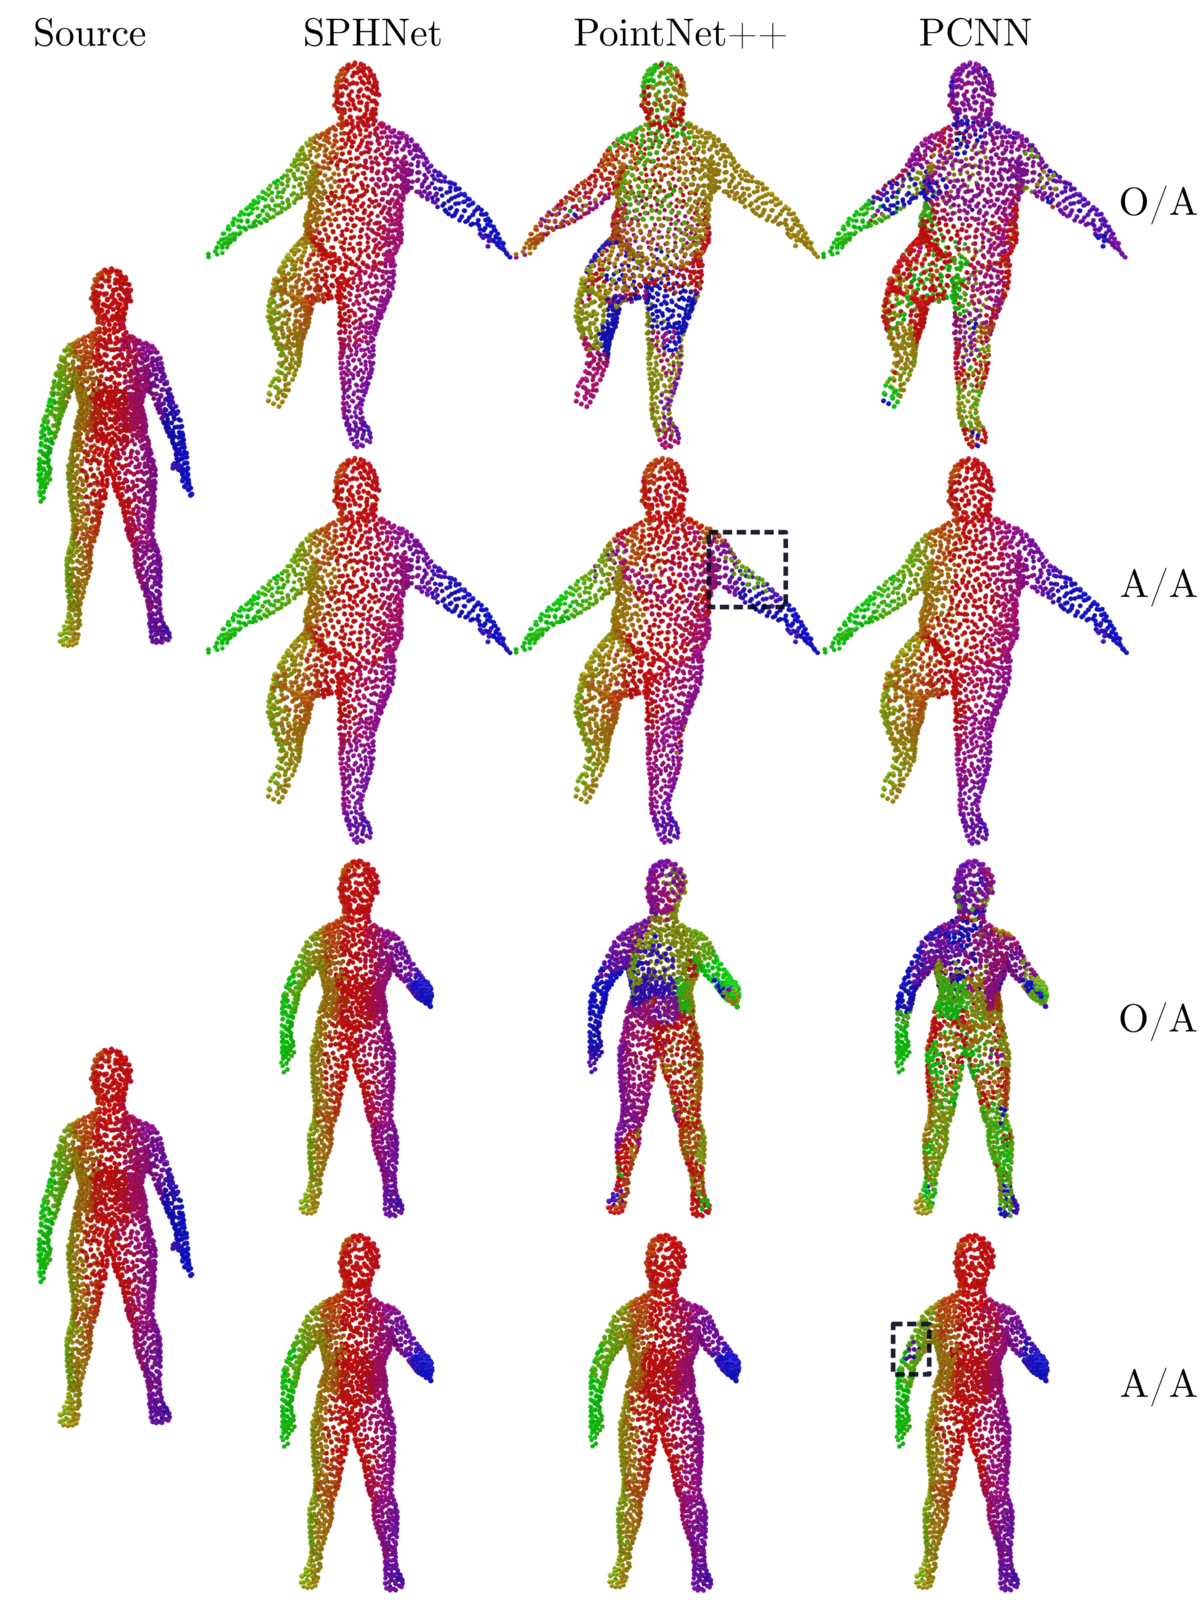}
    \caption{\revised{Qualitative comparison showing color map transfer inferred from Voronoi cell label predictions on two shape pairs from the DFAUST dataset. Note that our SPHNet method consistently produces smoother and more accurate maps both without (`O') and with (`A') data augmentation at training. }}
    \label{fig:dfaust_qual2}
\end{figure*}
